# Supplementary material for: Inverse Neural Rendering for Explainable Multi-Object Tracking
Source: arXiv:2404.12359 source file (2024-04-18)
Supplement: Supplementary file 1 [file fig_additional_nuscenes_results.tex]

\newpage
\begin{figure*}[h!]
	\vspace{-5pt}
	\centering
	\resizebox{0.98\linewidth}{!}{
	
	\begin{tabular}{@{}c@{\hskip 0.1cm}c@{\hskip 0.1cm}c@{\hskip 0.1cm}c@{\hskip 0.1cm}c@{\hskip 0.1cm}c@{}}
		\centering
            &
		{\huge Input $t_0$}&
		{\huge Tracked $t_0$}&
		{\huge Tracked $t_1$}&
		{\huge Tracked $t_2$}&
		{\huge Tracked $t_3$}\\

            \rotatebox[origin=c]{90}{{\Large	  Crossing 1}}&
		 \raisebox{-0.5\height}{\includegraphics[width=.38\columnwidth, trim={0cm 0cm 0cm 0cm},clip]{fig/additional_nuscenes_results/scene1/26_gt.png}}&
		 \raisebox{-0.5\height}{\includegraphics[width=.38\columnwidth, trim={0cm 0cm 0cm 0cm},clip]{fig/additional_nuscenes_results/scene1/26_bbox.png}}&
		 \raisebox{-0.5\height}{\includegraphics[width=.38\columnwidth, trim={0cm 0cm 0cm 0cm},clip]{fig/additional_nuscenes_results/scene1/27_bbox.png}}&
		 \raisebox{-0.5\height}{\includegraphics[width=.38\columnwidth, trim={0cm 0cm 0cm 0cm},clip]{fig/additional_nuscenes_results/scene1/28_bbox.png}}&
		 \raisebox{-0.5\height}{\includegraphics[width=.38\columnwidth, trim={0cm 0cm 0cm 0cm},clip]{fig/additional_nuscenes_results/scene1/29_bbox.png}}\\[1.9cm]
  
		\rotatebox[origin=c]{90}{{\Large	 Traffic}}&
		\raisebox{-0.5\height}{\includegraphics[width=.38\columnwidth, trim={0cm 0cm 0cm 0cm},clip]{fig/additional_nuscenes_results/scene13/gt_img.png}}&
		\raisebox{-0.5\height}{\includegraphics[width=.38\columnwidth, trim={0cm 0cm 0cm 0cm},clip]{fig/additional_nuscenes_results/scene13/23.png}} &
		\raisebox{-0.5\height}{\includegraphics[width=.38\columnwidth, trim={0cm 0cm 0cm 0cm},clip]{fig/additional_nuscenes_results/scene13/24.png}}&
		\raisebox{-0.5\height}{\includegraphics[width=.38\columnwidth, trim={0cm 0cm 0cm 0cm},clip]{fig/additional_nuscenes_results/scene13/25.png}}&
		\raisebox{-0.5\height}{\includegraphics[width=.38\columnwidth, trim={0cm 0cm 0cm 0cm},clip]{fig/additional_nuscenes_results/scene13/26.png}}\\[1.9cm]
  
            \rotatebox[origin=c]{90}{{\Large	Urban 1}}&
  		\raisebox{-0.5\height}{\includegraphics[width=.38\columnwidth, trim={0cm 0cm 0cm 0cm},clip]{fig/additional_nuscenes_results/scene12/gt.png}}&
		\raisebox{-0.5\height}{\includegraphics[width=.38\columnwidth, trim={0cm 0cm 0cm 0cm},clip]{fig/additional_nuscenes_results/scene12/21.png}}&
		\raisebox{-0.5\height}{\includegraphics[width=.38\columnwidth, trim={0cm 0cm 0cm 0cm},clip]{fig/additional_nuscenes_results/scene12/22.png}}&
		\raisebox{-0.5\height}{\includegraphics[width=.38\columnwidth, trim={0cm 0cm 0cm 0cm},clip]{fig/additional_nuscenes_results/scene12/23.png}}&
		\raisebox{-0.5\height}{\includegraphics[width=.38\columnwidth, trim={0cm 0cm 0cm 0cm},clip]{fig/additional_nuscenes_results/scene12/4.png}}\\[1.9cm]
  
            \rotatebox[origin=c]{90}{{\Large	Urban 2}}&
  		\raisebox{-0.5\height}{\includegraphics[width=.38\columnwidth, trim={0cm 0cm 0cm 0cm},clip]{fig/additional_nuscenes_results/scene4/2_gt.png}}&
		\raisebox{-0.5\height}{\includegraphics[width=.38\columnwidth, trim={0cm 0cm 0cm 0cm},clip]{fig/additional_nuscenes_results/scene4/2_out.png}}&
		\raisebox{-0.5\height}{\includegraphics[width=.38\columnwidth, trim={0cm 0cm 0cm 0cm},clip]{fig/additional_nuscenes_results/scene4/3_gt.png}}&
		\raisebox{-0.5\height}{\includegraphics[width=.38\columnwidth, trim={0cm 0cm 0cm 0cm},clip]{fig/additional_nuscenes_results/scene4/4_gt.png}}&
		\raisebox{-0.5\height}{\includegraphics[width=.38\columnwidth, trim={0cm 0cm 0cm 0cm},clip]{fig/additional_nuscenes_results/scene4/5_out.png}}\\[1.9cm]

        \rotatebox[origin=c]{90}{{\Large	 Urban 3}}&
		 \raisebox{-0.5\height}{\includegraphics[width=.38\columnwidth, trim={0cm 0cm 0cm 0cm},clip]{fig/additional_nuscenes_results/scene5/0783_0_gt.png}}&
		 \raisebox{-0.5\height}{\includegraphics[width=.38\columnwidth, trim={0cm 0cm 0cm 0cm},clip]{fig/additional_nuscenes_results/scene5/0783_0_bbox.png}}&
		 \raisebox{-0.5\height}{\includegraphics[width=.38\columnwidth, trim={0cm 0cm 0cm 0cm},clip]{fig/additional_nuscenes_results/scene5/0783_1_bbox.png}}&
		 \raisebox{-0.5\height}{\includegraphics[width=.38\columnwidth, trim={0cm 0cm 0cm 0cm},clip]{fig/additional_nuscenes_results/scene5/0783_2_bbox.png}}&
		 \raisebox{-0.5\height}{\includegraphics[width=.38\columnwidth, trim={0cm 0cm 0cm 0cm},clip]{fig/additional_nuscenes_results/scene5/0783_3_bbox.png}}\\[1.9cm]
        
    \rotatebox[origin=c]{90}{{\Large	  Crossing}}&
		 \raisebox{-0.5\height}{\includegraphics[width=.38\columnwidth, trim={0cm 0cm 0cm 0cm},clip]{fig/additional_nuscenes_results/scene6/0104_8_gt.png}}&
		 \raisebox{-0.5\height}{\includegraphics[width=.38\columnwidth, trim={0cm 0cm 0cm 0cm},clip]{fig/additional_nuscenes_results/scene6/0104_8_bbox.png}}&
		 \raisebox{-0.5\height}{\includegraphics[width=.38\columnwidth, trim={0cm 0cm 0cm 0cm},clip]{fig/additional_nuscenes_results/scene6/0104_9_bbox.png}}&
		 \raisebox{-0.5\height}{\includegraphics[width=.38\columnwidth, trim={0cm 0cm 0cm 0cm},clip]{fig/additional_nuscenes_results/scene6/0104_10_bbox.png}}&
		 \raisebox{-0.5\height}{\includegraphics[width=.38\columnwidth, trim={0cm 0cm 0cm 0cm},clip]{fig/additional_nuscenes_results/scene6/0104_11_bbox.png}}\\[1.9cm]

    \rotatebox[origin=c]{90}{{\Large	  Crossing 2}}&
		 \raisebox{-0.5\height}{\includegraphics[width=.38\columnwidth, trim={0cm 0cm 0cm 0cm},clip]{fig/additional_nuscenes_results/scene11/gt_img.png}}&
		 \raisebox{-0.5\height}{\includegraphics[width=.38\columnwidth, trim={0cm 0cm 0cm 0cm},clip]{fig/additional_nuscenes_results/scene11/27.png}}&
		 \raisebox{-0.5\height}{\includegraphics[width=.38\columnwidth, trim={0cm 0cm 0cm 0cm},clip]{fig/additional_nuscenes_results/scene11/28.png}}&
		 \raisebox{-0.5\height}{\includegraphics[width=.38\columnwidth, trim={0cm 0cm 0cm 0cm},clip]{fig/additional_nuscenes_results/scene11/29.png}}&
		 \raisebox{-0.5\height}{\includegraphics[width=.38\columnwidth, trim={0cm 0cm 0cm 0cm},clip]{fig/additional_nuscenes_results/scene11/30.png}}\\[1.9cm]

  \rotatebox[origin=c]{90}{{\Large	  Left View}}&
		 \raisebox{-0.5\height}{\includegraphics[width=.38\columnwidth, trim={0cm 0cm 0cm 0cm},clip]{fig/additional_nuscenes_results/scene9/gt_img.png}}&
		 \raisebox{-0.5\height}{\includegraphics[width=.38\columnwidth, trim={0cm 0cm 0cm 0cm},clip]{fig/additional_nuscenes_results/scene9/14.png}}&
		 \raisebox{-0.5\height}{\includegraphics[width=.38\columnwidth, trim={0cm 0cm 0cm 0cm},clip]{fig/additional_nuscenes_results/scene9/15.png}}&
		 \raisebox{-0.5\height}{\includegraphics[width=.38\columnwidth, trim={0cm 0cm 0cm 0cm},clip]{fig/additional_nuscenes_results/scene9/16.png}}&
		 \raisebox{-0.5\height}{\includegraphics[width=.38\columnwidth, trim={0cm 0cm 0cm 0cm},clip]{fig/additional_nuscenes_results/scene9/17.png}}\\[1.9cm]

 \rotatebox[origin=c]{90}{{\Large	Parking}}&
		 \raisebox{-0.5\height}{\includegraphics[width=.38\columnwidth, trim={0cm 0cm 0cm 0cm},clip]{fig/additional_nuscenes_results/scene10/gt_img.png}}&
		 \raisebox{-0.5\height}{\includegraphics[width=.38\columnwidth, trim={0cm 0cm 0cm 0cm},clip]{fig/additional_nuscenes_results/scene10/29.png}}&
		 \raisebox{-0.5\height}{\includegraphics[width=.38\columnwidth, trim={0cm 0cm 0cm 0cm},clip]{fig/additional_nuscenes_results/scene10/30.png}}&
		 \raisebox{-0.5\height}{\includegraphics[width=.38\columnwidth, trim={0cm 0cm 0cm 0cm},clip]{fig/additional_nuscenes_results/scene10/31.png}}&
		 \raisebox{-0.5\height}{\includegraphics[width=.38\columnwidth, trim={0cm 0cm 0cm 0cm},clip]{fig/additional_nuscenes_results/scene10/32.png}}\\[1.9cm]

  \rotatebox[origin=c]{90}{{\Large	  River}}&
		 \raisebox{-0.5\height}{\includegraphics[width=.38\columnwidth, trim={0cm 0cm 0cm 0cm},clip]{fig/additional_nuscenes_results/scene8/0_gt_new.png}}&
		 \raisebox{-0.5\height}{\includegraphics[width=.38\columnwidth, trim={0cm 0cm 0cm 0cm},clip]{fig/additional_nuscenes_results/scene8/0_new_bbox.png}}&
		 \raisebox{-0.5\height}{\includegraphics[width=.38\columnwidth, trim={0cm 0cm 0cm 0cm},clip]{fig/additional_nuscenes_results/scene8/1_new_bbox.png}}&
		 \raisebox{-0.5\height}{\includegraphics[width=.38\columnwidth, trim={0cm 0cm 0cm 0cm},clip]{fig/additional_nuscenes_results/scene8/bbox_2_new.png}}&
		 \raisebox{-0.5\height}{\includegraphics[width=.38\columnwidth, trim={0cm 0cm 0cm 0cm},clip]{fig/additional_nuscenes_results/scene8/bbox_3_new.png}}\\[1.9cm]

	\end{tabular}
	}
	\caption{Additional visualizations on nuScenes~\cite{caesar2020nuscenes}. From left to right, we show (i) observed images from diverse scenes at timestep $k=0$; (ii) an overlay of the optimized generated object and its 3D bounding boxes at timestep $k=0, 1, 2 \text{ and } 3$. The color of the bounding boxes for each object corresponds to the predicted tracklet ID. We see that our method can accurately reconstruct objects in diverse scenarios.}
	\label{fig:additional_nuScenes_results}

\end{figure*}
\newpage
